# Supplementary material for: RoboDepth: Robust Out-of-Distribution Depth Estimation under Corruptions
Source: arXiv:2310.15171 source file (2023-10-23)
Supplement: Supplementary file 1 [file calibration.tex]

\begin{table*}[t]
    \centering
    \caption{Depth estimation model calibration from different aspects (modality, backbone, pertaining strategy, and loss function).}
    \label{tab:calibration}
    \scalebox{0.66}{
    \begin{tabular}{r|c|c|c|c|c|c}
    \toprule
    \textbf{Model} & \textbf{Venue} & \textbf{Modality} & \textbf{Motivation} & \textbf{Backbone} & \textbf{Pretrain} & \textbf{Loss Function} 
    \\\midrule
    MonoDepth2 \cite{godard2019monodepth2} & ICCV'19 & Mono \& Stereo & Auto-masking \& multi-scale cues & ResNet-18/50 & ImageNet & photometric re-projection; per-pixel smoothness
    \\
    DepthHints \cite{watson2019hints} & ICCV'19 & Stereo & Complementary depth suggestions & ResNet-18 & ImageNet & photometric re-projection; per-pixel smoothness
    \\
    SC-Depth \cite{bian2019scdepth} & NeurIPS'19 & Mono & Geometry consistency constraint & ResNet-50 & CityScapes & consistency; photometric re-projection; smoothness
    \\
    CADepth \cite{yan2021cadepth} & 3DV'21 & Mono \& Stereo & Channel-wise  structural attention & ResNet-50 & ImageNet & photometric re-projection; per-pixel smoothness
    \\
    HR-Depth \cite{lyu2021hrdepth} & AAAI'21 & Mono & High-resolution features fusion & ResNet-18 & Cityscapes & photometric re-projection; per-pixel smoothness
    \\
    DIFFNet \cite{zhou2021diffnet} & BMVC'21 & Mono & Internel feature fusion mechanism & HRNet & ImageNet & photometric re-projection; per-pixel smoothness
    \\
    ManyDepth \cite{watson2021manydepth} & CVPR'21 & Multi-Mono & Sequential test-time information & ResNet-18 & ImageNet & consistency; photometric re-projection; smoothness
    \\
    FSRE-Depth \cite{jung2021fsre} & ICCV'21 & Mono & Semantics-guided triplet loss & ResNet-18 & ImageNet & semantic triplet; photometric re-projection; smoothness
    \\
    MonoViT \cite{zhao2021monovit} & 3DV'21 & Mono & Global reasoning via self-attention & MPViT & ImageNet & photometric re-projection; per-pixel smoothness
    \\
    DynaDepth \cite{zhang2022dynadepth} & ECCV'22 & Mono & Vision and IMU motion dynamics & ResNet-18/50 & ImageNet & IMU photometric; cross-sensor photometric consistency
    \\
    TriDepth \cite{chen2023tridepth} & WACV'23  & Multi-Mono & Patch-based triplet optimizing strategy & ResNet-18 & ImageNet & patch triplet; photometric re-projection; smoothness
    \\
    Lite-Mono \cite{zhang2023litemono} & CVPR'23 & Mono & Efficient mix of CNNs \& attentions & ResNet-18 & ImageNet & photometric re-projection; per-pixel smoothness
    \\\bottomrule
    \end{tabular}
    }
\end{table*}
